# Supplementary material for: Enhancing magnetic near-field intensities with dielectric resonators
Source: arXiv:1303.4794 source file (2013-07-30)
Supplement: Supplementary file 1 [file supplemental_material_VF.pdf]

# Supplemental Material for : Enhancing magnetic near–field intensities with dielectric resonators

Guillaume Boudarham,* Redha Abdeddaim, and Nicolas Bonod

*Institut Fresnel, CNRS, Aix-Marseille Université, Ecole Centrale Marseille Campus de Saint Jérôme, 13013 Marseille, France*

E-mail: guillaume.boudarham@fresnel.fr

**Abstract**

We detail the analytical derivation of the model used to calculate the magnetic field intensities inside a subwavelength dielectric dimer and we give the expressions of the dipolar moments of each particle of the dimer with respect to the incident field. The analytical results are compared to full numerical calculations obtained from a finite element method.

*To whom correspondence should be addressed

# Dipolar model for dimers

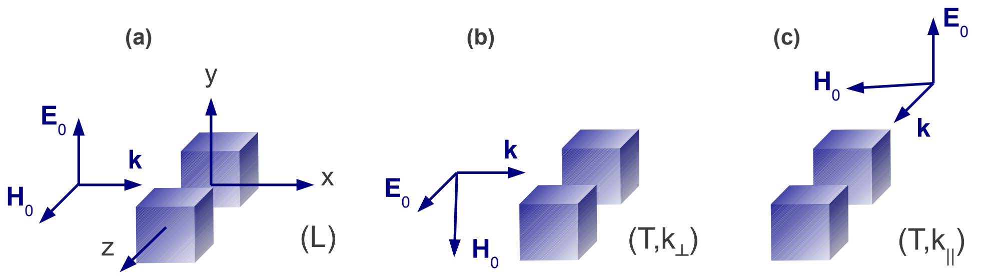


Figure 1: (Color online) Dimer illumination schematics for (a) longitudinal illumination and (b) and (c) transverse illuminations.

We derive below a general dipolar model which allows us to calculate the electric and magnetic dipolar moments of each particle of a dimer illuminated by a plane wave in arbitrary incidence. These moments can be used to calculate the electric and magnetic fields everywhere in space and especially inside the gap between the neighboring particles. In the following we use the international system of units.

We assume that the dimer is illuminated by a plane wave $(\boldsymbol{E}_0, \boldsymbol{H}_0)$ and for simplification, we will take $|\boldsymbol{E}_0| = 1(V/m)$ and thus $|\boldsymbol{H}_0| = 1/Z_0$, where $Z_0 = 376.730\,\Omega$ is the impedance of free space. We assume also that the dimensions of the dimer are small with respect to the incident wavelength, this will allow us to use the dipolar approximation.

Let us consider a dimer consisting of two particles located at positions $\boldsymbol{r}_n$ $(n = 1, 2)$. When the dimer is illuminated by a plane wave, it appears in each particle an electric dipole $\boldsymbol{p}_n$ and a magnetic dipole $\boldsymbol{m}_n$. We will assume that the particles of the dimer are identical, non-bianisotropic and described by the polarizability tensor $\bar{\bar{\boldsymbol{\alpha}}} = \mathrm{diag}(\bar{\bar{\boldsymbol{\alpha}}}_e, \bar{\bar{\boldsymbol{\alpha}}}_m)$. The dipolar moments verify the general system of equations[1] :

$$\begin{pmatrix} \boldsymbol{p}_n/\varepsilon_0 \\ \boldsymbol{m}_n \end{pmatrix} = \bar{\bar{\boldsymbol{\alpha}}} \cdot \left[ \begin{pmatrix} \boldsymbol{E}_0(\boldsymbol{r}_n) \\ \boldsymbol{H}_0(\boldsymbol{r}_n) \end{pmatrix} + \sum_{\substack{q=1,2 \\ q\neq n}} \bar{\bar{\boldsymbol{G}}}^0(\boldsymbol{r}_n, \boldsymbol{r}_q) \cdot \begin{pmatrix} \boldsymbol{p}_q \\ \boldsymbol{m}_q \end{pmatrix} \right], \tag{1}$$

where

$$\bar{\bar{\boldsymbol{G}}}^0(\boldsymbol{r}, \boldsymbol{r}') = \begin{pmatrix} \bar{\bar{\boldsymbol{G}}}^0_{ee}(\boldsymbol{r}, \boldsymbol{r}') & \bar{\bar{\boldsymbol{G}}}^0_{em}(\boldsymbol{r}, \boldsymbol{r}') \\ \bar{\bar{\boldsymbol{G}}}^0_{me}(\boldsymbol{r}, \boldsymbol{r}') & \bar{\bar{\boldsymbol{G}}}^0_{mm}(\boldsymbol{r}, \boldsymbol{r}') \end{pmatrix} \tag{2}$$

is the full dyadic Green's function of free space. The $3 \times 3$ diagonal blocks correspond to the well-known electric and magnetic dyadic Green's functions of free space[2]. The off-diagonal blocks correspond to the mixed dyadics that give the electric field at $\boldsymbol{r}$ due to a magnetic dipole at $\boldsymbol{r}'$ and the magnetic field at $\boldsymbol{r}$ due to an electric dipole at $\boldsymbol{r}'$. $\boldsymbol{E}_0(\boldsymbol{r}_n)$ and $\boldsymbol{H}_0(\boldsymbol{r}_n)$ respectively denote the incident electric and magnetic field at $\boldsymbol{r}_n$. The second term in brackets represents the field scattered by the other particle.

We assume that the electric and magnetic polarizability tensors of the individual particles are diagonal and they can be described by scalars : $\bar{\bar{\boldsymbol{\alpha}}}_e = \alpha_e \text{diag}(1,1,1)$ and $\bar{\bar{\boldsymbol{\alpha}}}_m = \alpha_m \text{diag}(1,1,1)$. Note that $\alpha_e$ and $\alpha_m$ can be calculated from the knowledge of the polarization density of the individual particles. In this work, they have been calculated by using a finite element method implemented in COMSOL Multiphysics.

## Calculation of the dipolar moments

To calculate the dipolar moments of each particle of the dimer for any the illumination conditions, we write Eq. (1) in matrix form :

$$\bar{\bar{\boldsymbol{M}}}.\boldsymbol{D} = \boldsymbol{F}, \tag{3}$$

where

$$\bar{\bar{\boldsymbol{M}}} \equiv \begin{pmatrix} \bar{\bar{\boldsymbol{I}}} & -\varepsilon_0\alpha_e\bar{\bar{\boldsymbol{G}}}^0_{ee}(\boldsymbol{r}_1,\boldsymbol{r}_2) & \boldsymbol{0} & -\varepsilon_0\alpha_e\bar{\bar{\boldsymbol{G}}}^0_{em}(\boldsymbol{r}_1,\boldsymbol{r}_2) \\ -\varepsilon_0\alpha_e\bar{\bar{\boldsymbol{G}}}^0_{ee}(\boldsymbol{r}_2,\boldsymbol{r}_1) & \bar{\bar{\boldsymbol{I}}} & -\varepsilon_0\alpha_e\bar{\bar{\boldsymbol{G}}}^0_{em}(\boldsymbol{r}_2,\boldsymbol{r}_1) & \boldsymbol{0} \\ \boldsymbol{0} & -\alpha_m\bar{\bar{\boldsymbol{G}}}^0_{me}(\boldsymbol{r}_1,\boldsymbol{r}_2) & \bar{\bar{\boldsymbol{I}}} & -\alpha_m\bar{\bar{\boldsymbol{G}}}^0_{mm}(\boldsymbol{r}_1,\boldsymbol{r}_2) \\ -\alpha_m\bar{\bar{\boldsymbol{G}}}^0_{me}(\boldsymbol{r}_2,\boldsymbol{r}_1) & \boldsymbol{0} & -\alpha_m\bar{\bar{\boldsymbol{G}}}^0_{mm}(\boldsymbol{r}_2,\boldsymbol{r}_1) & \bar{\bar{\boldsymbol{I}}} \end{pmatrix}, \quad (4)$$

$$\boldsymbol{D} \equiv \begin{pmatrix} \boldsymbol{p}_1 \\ \boldsymbol{p}_2 \\ \boldsymbol{m}_1 \\ \boldsymbol{m}_2 \end{pmatrix}, \ \boldsymbol{F} \equiv \begin{pmatrix} \varepsilon_0\alpha_e\boldsymbol{E}_0(\boldsymbol{r}_1) \\ \varepsilon_0\alpha_e\boldsymbol{E}_0(\boldsymbol{r}_2) \\ \alpha_m\boldsymbol{H}_0(\boldsymbol{r}_1) \\ \alpha_m\boldsymbol{H}_0(\boldsymbol{r}_2) \end{pmatrix}, \quad (5)$$

$\bar{\bar{\boldsymbol{M}}}$ is a $12\times 12$ block matrix, $\bar{\bar{\boldsymbol{I}}} = \mathrm{diag}(1,1,1)$ and $\boldsymbol{0}$ respectively denote the $3\times 3$ unit dyadic and the dyadic filled with zeros. The vector $\boldsymbol{D}$ describes the dipolar moments of each particle and the vector $\boldsymbol{F}$ is linked to the incident electromagnetic field in the particles[3]. The origin of the coordinate system is chosen at the center of the dimer and the $z$-axis is parallel to the dimer axis. We obtain :

$$\bar{\bar{\boldsymbol{G}}}^0_{ee}(\boldsymbol{r}_1,\boldsymbol{r}_2) = \begin{pmatrix} G^0_{ee,xx} & 0 & 0 \\ 0 & G^0_{ee,yy} & 0 \\ 0 & 0 & G^0_{ee,zz} \end{pmatrix}, \qquad \bar{\bar{\boldsymbol{G}}}^0_{em}(\boldsymbol{r}_1,\boldsymbol{r}_2) = \begin{pmatrix} 0 & G^0_{em,xy} & 0 \\ G^0_{em,yx} & 0 & 0 \\ 0 & 0 & 0 \end{pmatrix}$$

$$\bar{\bar{\boldsymbol{G}}}^0_{me}(\boldsymbol{r}_1,\boldsymbol{r}_2) = \begin{pmatrix} 0 & G^0_{me,xy} & 0 \\ G^0_{me,yx} & 0 & 0 \\ 0 & 0 & 0 \end{pmatrix}, \qquad \bar{\bar{\boldsymbol{G}}}^0_{mm}(\boldsymbol{r}_1,\boldsymbol{r}_2) = \begin{pmatrix} G^0_{mm,xx} & 0 & 0 \\ 0 & G^0_{mm,yy} & 0 \\ 0 & 0 & G^0_{mm,zz} \end{pmatrix}$$

with

$$G^0_{ee,xx} = \frac{e^{ikd}}{4\pi\varepsilon_0 d^3}(k^2d^2 + ikd - 1), \qquad G^0_{ee,zz} = \frac{e^{ikd}}{2\pi\varepsilon_0 d^3}(1 - ikd)$$

$$G^0_{em,yx} = \mu_0 \frac{e^{ikd}}{4\pi d} k\omega(1 + \frac{i}{kd}), \qquad G^0_{mm,xx} = \frac{e^{ikd}}{4\pi d^3}(k^2d^2 + ikd - 1)$$

$$G^0_{mm,zz} = \frac{e^{ikd}}{2\pi d^3}(1 - ikd), \qquad G^0_{me,xy} = \frac{e^{ikd}}{4\pi d} k\omega(1 + \frac{i}{kd})$$

where $d = |\boldsymbol{r}_2 - \boldsymbol{r}_1|$ is the distance between the dipoles, found to be located at the center of the particles. Also we find the relations :

$$G^0_{ee,xx} = G^0_{ee,yy}, \qquad G^0_{mm,xx} = G^0_{mm,yy}$$

$$G^0_{em,yx} = -G^0_{em,xy}, \qquad G^0_{me,yx} = -G^0_{me,xy}$$

and

$$\bar{\bar{\boldsymbol{G}}}^0_{ee}(\boldsymbol{r}_2, \boldsymbol{r}_1) = \bar{\bar{\boldsymbol{G}}}^0_{ee}(\boldsymbol{r}_1, \boldsymbol{r}_2), \qquad \bar{\bar{\boldsymbol{G}}}^0_{mm}(\boldsymbol{r}_2, \boldsymbol{r}_1) = \bar{\bar{\boldsymbol{G}}}^0_{mm}(\boldsymbol{r}_1, \boldsymbol{r}_2)$$

$$\bar{\bar{\boldsymbol{G}}}^0_{em}(\boldsymbol{r}_2, \boldsymbol{r}_1) = \left[\bar{\bar{\boldsymbol{G}}}^0_{em}(\boldsymbol{r}_1, \boldsymbol{r}_2)\right]^T, \qquad \bar{\bar{\boldsymbol{G}}}^0_{me}(\boldsymbol{r}_2, \boldsymbol{r}_1) = \left[\bar{\bar{\boldsymbol{G}}}^0_{me}(\boldsymbol{r}_1, \boldsymbol{r}_2)\right]^T.$$

Expression (3) shows that the dipolar moments of each particle can be obtained by inverting the matrix $\bar{\bar{\boldsymbol{M}}}$ :

$$\boldsymbol{D} = \bar{\bar{\boldsymbol{M}}}^{-1}.\boldsymbol{F}. \tag{6}$$

We used the symbolic math toolbox of MathWorks to formally invert this matrix. It is a $12 \times 12$ matrix whose elements could be calculated as functions of $d$ and the incident frequency.

## Expressions of the dipolar moments

Three illuminations are considered to illuminate the dimer of cubes for which either the incident magnetic or electric field or the incident wavevector is parallel to the dimer axis (see Fig. 1):

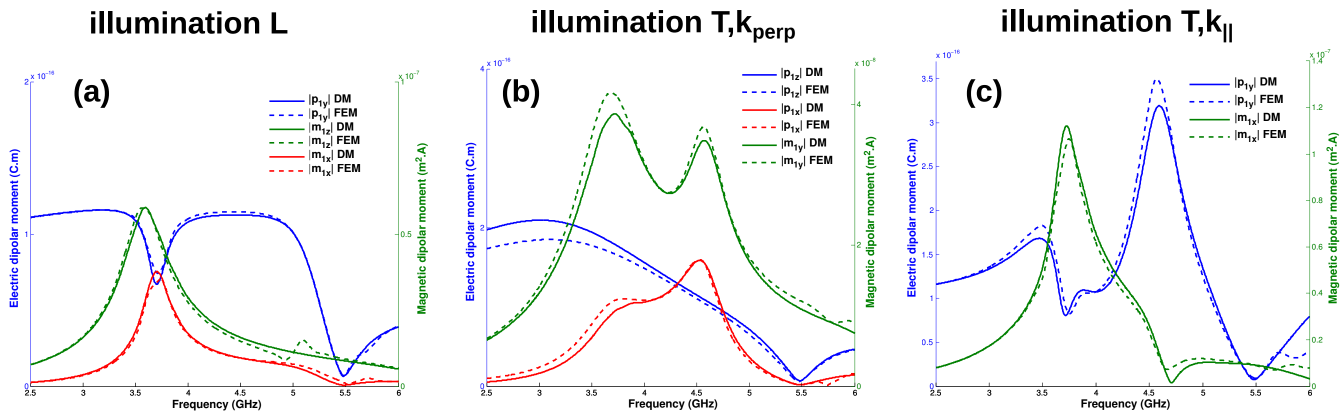


Figure 2: (Color online) Modulus of the dipolar moments obtained from the dipolar model (DM) and compared to a FEM analysis for a gap size of 4 mm.

$$\boldsymbol{H}_{0,L}(x) = |\boldsymbol{H}_0| e^{ikx} \hat{\boldsymbol{e}}_z, \tag{7}$$

$$\boldsymbol{H}_{0,T,k_\perp}(x) = -|\boldsymbol{H}_0| e^{ikx} \hat{\boldsymbol{e}}_y, \tag{8}$$

$$\boldsymbol{H}_{0,T,k_\parallel}(z) = -|\boldsymbol{H}_0| e^{ikz} \hat{\boldsymbol{e}}_x. \tag{9}$$

In the following we give the explicit expressions of the non-vanishing dipolar moments.

**Longitudinal illumination**

$$m_{1z} = m_{2z} = \frac{\alpha_m |\boldsymbol{H}_0|}{1+\gamma_4}; \qquad m_{1x} = -m_{2x} = \frac{\varepsilon_0 \alpha_e |\boldsymbol{E}_0| \gamma_5}{\gamma_3 - \gamma_2\gamma_5 + \gamma_1(\gamma_3 - 1) - 1};$$

and

$$p_{1y} = p_{2y} = \frac{\varepsilon_0 \alpha_e |\boldsymbol{E}_0| (\gamma_3 - 1)}{\gamma_3 - \gamma_2\gamma_5 + \gamma_1(\gamma_3 - 1) - 1}, \tag{10}$$

where

$$\gamma_1 \equiv -\frac{\alpha_e}{4\pi l^3} e^{ikl}(k^2 l^2 + ikl - 1); \qquad \gamma_2 \equiv -\alpha_e \varepsilon_0 \frac{\mu_0}{4\pi l} e^{ikl} k\omega \left(1 + \frac{i}{kl}\right);$$

$$\gamma_3 \equiv -\frac{\alpha_m}{4\pi l^3} e^{ikl}(k^2 l^2 + ikl - 1); \qquad \gamma_4 \equiv -\frac{\alpha_m}{2\pi l^3} e^{ikl}(1 - ikl)$$

and

$$\gamma_5 \equiv -\frac{\alpha_m}{4\pi l} e^{ikl} k\omega \left(1 + \frac{i}{kl}\right). \tag{11}$$

$\gamma_1$ and $\gamma_4$ represent the transverse and longitudinal inter-particle scattering for the electric and the magnetic field respectively. They take into account the electric and magnetic fields scattered in one particle by the electric and magnetic dipolar moments of the other particle respectively. $\gamma_2$ and $\gamma_5$ are cross-coupling terms which take into account the electric and magnetic fields scattered in one particle by the magnetic and electric dipolar moment of the other particle respectively.

The cross-coupling term $\gamma_5$ implies that the direction of the magnetic dipolar moments does not coincide with the direction of the incident magnetic field ($z$-axis), while the electric dipolar moment remains parallel to the incident electric field ($y$-axis). This result comes from the fact that in a magneto-electric dimer, a $x$-component of the magnetic dipolar moment in one cube can be feeded by the magnetic field scattered by the $y$-component of the electric dipolar moment of the neighboring cube. We note that the electric response is driven electrically only, while the magnetic response is driven in part magnetically, and in part electrically. The asymmetry observed for the dipolar moments results from the asymmetry of the illuminating field (the electric field is polarized along the $y$-axis) and it does not violate the so-called Onsager constraints[4].

Fig. 2 (a) shows the dipolar moments $m_{1z}$, $m_{1x}$ and $p_{1y}$ obtained from Eqs. (10) for a gap size of 4 mm. Also, we observe an anti-resonance in the modulus of $p_{1y}$ (blue line) at 3.71 GHz which coincides with a resonance of the modulus of $m_{1x}$ (red line). This anti-resonance is a manifestation of the cross-coupling between the electric and magnetic dipolar moments of each resonator and it disappears if we set formally $\gamma_5 = 0$ (or $\gamma_2 = 0$).

**Transverse $T, k_\perp$ illumination**

$$p_{1x} = -p_{2x} = \frac{\alpha_m |\boldsymbol{H}_0| \gamma_2}{\gamma_1 - \gamma_2\gamma_5 + \gamma_3(\gamma_1 - 1) - 1}; \qquad p_{1z} = p_{2z} = \frac{\varepsilon_0 \alpha_e |\boldsymbol{E}_0|}{1 + \gamma_6};$$

and

$$m_{1y} = m_{2y} = -\frac{\alpha_m |\boldsymbol{H}_0| (\gamma_1 - 1)}{\gamma_1 - \gamma_2\gamma_5 + \gamma_3(\gamma_1 - 1) - 1}, \tag{12}$$

where $\gamma_1$, $\gamma_2$, $\gamma_3$ and $\gamma_5$ have been defined previously and

$$\gamma_6 \equiv -\frac{\alpha_e}{2\pi l^3} e^{ikl}(1 - ikl). \tag{13}$$

The cross-coupling term $\gamma_2$ implies that the direction of the electric dipolar moments does not coincide with the direction of the incident electric field ($z$-axis), while the magnetic dipolar moment remains parallel to the incident magnetic field ($y$-axis). This result comes from the fact that in a magneto-electric dimer, a $x$-component of the electric dipolar moment in one cube can be feeded by the electric field scattered by the $y$-component of the magnetic dipolar moment of the neighboring cube. Fig. 2 (b) shows the dipolar moments $p_{1x}$, $p_{1z}$ and $m_{1y}$ obtained from Eqs. (12) for a gap size of 4 mm.

**Transverse $T, k_\parallel$ illumination**

$$p_{1y} = \frac{P_1 + \gamma_5(P_1\gamma_2 + M_2\gamma_2^2 - P_2\gamma_2\gamma_3) + M_2\gamma_2 - \gamma_1(-P_2\gamma_3^2 + M_2\gamma_2\gamma_3 + P_2 - M_1\gamma_2) - P_1\gamma_3^2 - M_1\gamma_2\gamma_3}{\gamma_1^2\gamma_3^2 - \gamma_1^2 - 2\gamma_1\gamma_2\gamma_3\gamma_5 + \gamma_2^2\gamma_5^2 + 2\gamma_2\gamma_5 - \gamma_3^2 + 1}; \tag{14}$$

$$p_{2y} = -\frac{\gamma_5(M_1\gamma_2^2 - P_2\gamma_2 + P_1\gamma_2\gamma_3) - P_2 + M_1\gamma_2 + \gamma_1(-P_1\gamma_3^2 - M_1\gamma_2\gamma_3 + P_1 + M_2\gamma_2) + P_2\gamma_3^2 - M_2\gamma_2\gamma_3}{\gamma_1^2\gamma_3^2 - \gamma_1^2 - 2\gamma_1\gamma_2\gamma_3\gamma_5 + \gamma_2^2\gamma_5^2 + 2\gamma_2\gamma_5 - \gamma_3^2 + 1}; \tag{15}$$

$$m_{1x} = -\frac{M_1 + \gamma_2(M_1\gamma_5 + P_2\gamma_5^2 - M_2\gamma_1\gamma_5) + P_2\gamma_5 - \gamma_3(-M_2\gamma_1^2 + P_2\gamma_1\gamma_5 + M_2 - P_1\gamma_5) - M_1\gamma_1^2 - P_1\gamma_1\gamma_5}{\gamma_1^2\gamma_3^2 - \gamma_1^2 - 2\gamma_1\gamma_2\gamma_3\gamma_5 + \gamma_2^2\gamma_5^2 + 2\gamma_2\gamma_5 - \gamma_3^2 + 1}; \tag{16}$$

$$m_{2x} = \frac{\gamma_2(P_1\gamma_5^2 - M_2\gamma_5 + M_1\gamma_1\gamma_5) - M_2 + P_1\gamma_5 + \gamma_3(-M_1\gamma_1^2 - P_1\gamma_1\gamma_5 + M_1 + P_2\gamma_5) + M_2\gamma_1^2 - P_2\gamma_1\gamma_5}{\gamma_1^2\gamma_3^2 - \gamma_1^2 - 2\gamma_1\gamma_2\gamma_3\gamma_5 + \gamma_2^2\gamma_5^2 + 2\gamma_2\gamma_5 - \gamma_3^2 + 1}, \tag{17}$$

where

$$P_1 \equiv |\boldsymbol{E}_0|\varepsilon_0\alpha_e e^{-ikl}, \;\; M_1 \equiv |\boldsymbol{H}_0|\alpha_m e^{-ikl} \tag{18}$$

$$P_2 \equiv |\boldsymbol{E}_0|\varepsilon_0\alpha_e e^{ikl}, \;\; M_2 \equiv |\boldsymbol{H}_0|\alpha_m e^{ikl}. \tag{19}$$

In this illumination condition, Eqs. (14)-(17) show that the electric and magnetic dipolar moments of each particle are aligned with the incident electric and magnetic field respectively. Fig. 2 (c) shows the dipolar moments $p_{1y}$, $p_{2y}$, $m_{1x}$, $m_{2x}$ as a function of the frequency for a gap size of 4 mm.

# Magnetic near field as a function of the frequency and gap size

We show in 3 the normalized magnetic field intensity as a function of both the gap size the illuminating frequency obtained from the dipolar model.

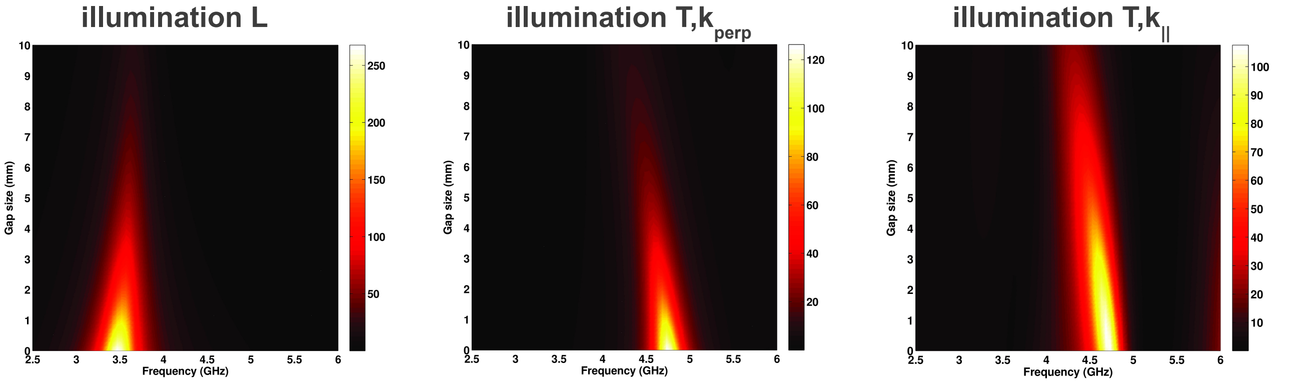


Figure 3: (Color online) Normalized magnetic field intensity as a function of the frequency and gap size for the three conditions of illumination considered in this work.

Similarly to metallic dimer antennas that allow for strong near electric fields when the incident electric field is parallel to the dimer axis, for the longitudinal illumination, the coupling of the magnetic modes leads to a redshift of the resonance[5] but we observe a blueshift of the resonance when either the incident electric field or the wave vector is parallel to the dimer axis. Also, we observe that the magnetic field intensity increases as the gap size decreases. This result implies that it is possible to obtain a magnetic enhancement more important than that obtained with a gap size of 5 mm even further reducing the distance between the resonators for the three conditions of illumination considered here.

# Electric near field in the center of the dimer

For the three conditions of illumination, the normalized electric field intensity could not be measured experimentally but it was obtained from the dipolar model and a FEM analysis.

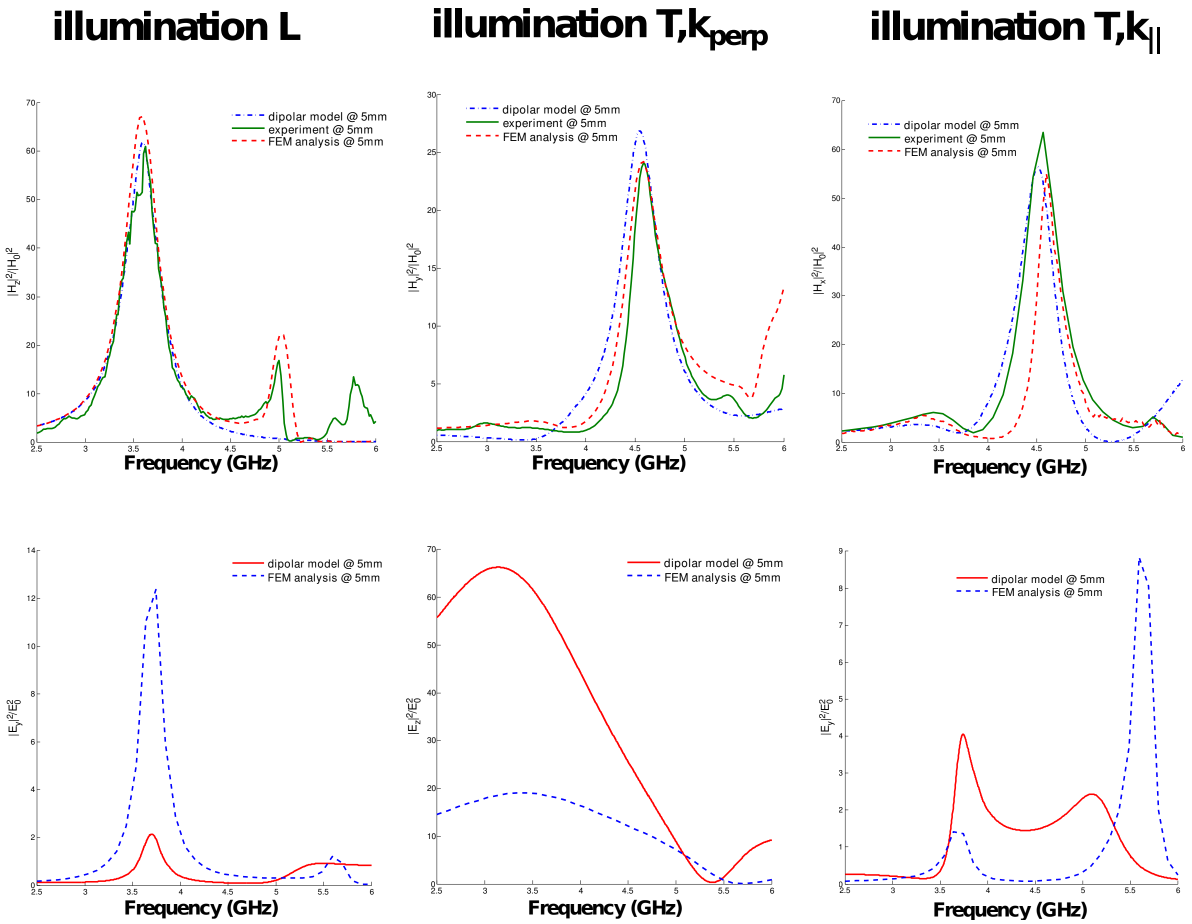


Figure 4: (Color online) On top : normalized magnetic field intensity in the center of the gap of the dimer for a gap size of 5 mm obtained from the dipolar model, experiments and a FEM analysis. At the bottom : normalized electric field intensity obtained from the dipolar model and a FEM analysis.

We give below the expressions of the electric field at the center of the gap of the dimer for the three conditions of illuminations considered in this work :

$$
\begin{aligned}
E_{y,L} &= \frac{e^{ikl}}{4\pi\varepsilon_0 l^3}(k^2l^2+ikl-1)p_{1y}+\frac{e^{ikl}}{4\pi\varepsilon_0 l^3}(k^2l^2+ikl-1)p_{2y} \\
&- \frac{e^{ikl}}{4\pi\varepsilon_0 c l^3}(k^2l^2+ikl)m_{1x}+\frac{e^{ikl}}{4\pi\varepsilon_0 c l^3}(k^2l^2+ikl)m_{2x};
\end{aligned}
\qquad (20)
$$

$$E_{z,T,k_\perp} = \frac{e^{ikl}}{2\pi\varepsilon_0 l^3}(1-ikl)p_{1z} + \frac{e^{ikl}}{2\pi\varepsilon_0 l^3}(1-ikl)p_{2z}; \qquad (21)$$

$$\begin{aligned} E_{y,T,k_\parallel} &= \frac{e^{ikl}}{4\pi\varepsilon_0 l^3}(k^2l^2+ikl-1)p_{1y} + \frac{e^{ikl}}{4\pi\varepsilon_0 l^3}(k^2l^2+ikl-1)p_{2y} \\ &- \frac{e^{ikl}}{4\pi\varepsilon_0 c l^3}(k^2l^2+ikl)m_{1x} + \frac{e^{ikl}}{4\pi\varepsilon_0 c l^3}(k^2l^2+ikl)m_{2x}. \end{aligned} \qquad (22)$$

We show in Fig. 4 at the bottom the normalized electric field intensity in the center of the gap of the dimer for a gap size of 5 mm obtained from a FEM analysis and compared to those obtained from the dipolar model [see Eqs. (20)-(22)]. One can see that the maximum electric enhancement is always less than an order of magnitude, which is very weak compared to enhancement reported with the magnetic field intensity for an identical gap size. Unlike the results obtained for the magnetic field (see Fig. 4 on top), one can see a significant difference between the results obtained from the analytical model and those obtained from a FEM analysis for the three conditions of illuminations. These differences are due to the excitation of the electric quadrupole which is not taken into account in the model.

## References


(1) De Abajo, F. G. *Reviews of modern physics* **2007**, *79*, 1267.

(2) Novotny, L.; Hecht, B. *Principles of Nano-Optics*; Cambridge University Press, 2006.

(3) Jackson, J. D. *Classical Electrodynamics : Third Edition*; John Wiley & Sons: New York, 1999.

(4) Sersic, I.; Tuambilangana, C.; Kampfrath, T.; Koenderink, A. F. *Physical Review B: Condensed Matter and Materials Physics* **2011**, *83*, 245102.

(5) Busson, M. P.; Rolly, B.; Stout, B.; Bonod, N.; Larquet, E.; Polman, A.; Bidault, S. *Nano Letters* **2011**, *11*, 5060–5065.
